# Supplementary material for: Group-based Robustness: A General Framework for Customized Robustness in the Real World
Source: arXiv:2306.16614 source file (2024-03-10)
Supplement: Supplementary file 1 [file appendix.tex]

\section{Appendix}
\label{sec:appendix}
